# Supplementary material for: Succinct Classical Verification of Quantum Computation
Source: arXiv:2206.14929 source file (2022-06-29)
Supplement: Supplementary file 1 [file appendix-isometry.tex]

\section{Implementing the Isometry}
\label{sec:isometry-circuit}

We now show how to implement $V$ efficiently given black-box (as in \cref{subsec:black-box}) access to $\{X(r), Z(s)\}$. Let $U_{\textrm{Bell}}$ be the unitary that computes the outcome of the $N$ Bell basis measurements onto a $2N$-qubit ancilla register, i.e., for all $r,s,r',s' \in \{0,1\}^{N}$,
\[ U_{\textrm{Bell}}\left(\ket{\phi^{r,s}} \otimes \ket{r',s'}\right) \coloneqq \ket{\phi^{r,s}} \otimes \ket{r \oplus r',s \oplus s'}.\]

The following quantum circuit acting on $\RegH,\RegA_1,\RegA_2$ and an additional $2N$-qubit ancilla implements $V$ when $\RegH$ is initialized to $\ket{\psi}$, and $\RegA_1 \otimes \RegA_2$ is initialized to $\dfrac{1}{2^N}\displaystyle\sum_{r,s \in \{0,1\}^N} \ket{\phi^{r,s}}_{\RegA_1,\RegA_2}$, the uniform superposition over the states $\{\ket{\phi^{r,s}}\}_{r,s \in \{0,1\}^{N}}$.\\

\begin{quantikz}
\lstick[wires=1]{$\ket{\psi}_{\RegH}$} & \qwbundle[alternate]{} & \gate[wires=1]{X(r)Z(s)}\qwbundle[alternate]{} & \qwbundle[alternate]{} & \rstick[wires=3]{$V(\ket{\psi})_{\RegH,\RegA_1,\RegA_2}$}\qwbundle[alternate]{} \\
\lstick[wires=2]{$\dfrac{1}{2^N}\displaystyle\sum_{r,s \in \{0,1\}^N} \ket{\phi^{r,s}}_{\RegA_1,\RegA_2}$} & \gate[wires=3]{U_{\textrm{Bell}}}\qwbundle[alternate]{} & \qwbundle[alternate]{} & \gate[wires=3]{U_{\textrm{Bell}}}\qwbundle[alternate]{} & \qwbundle[alternate]{} \\
& \qwbundle[alternate]{} & \qwbundle[alternate]{} & \qwbundle[alternate]{} & \qwbundle[alternate]{} \\
\lstick[wires=1]{$\ket{0^{2N}}$} & \qwbundle[alternate]{} &  \ctrlbundle{-3}\qwbundle[alternate]{}  & \qwbundle[alternate]{} & \qwbundle[alternate]{} \\
\end{quantikz}
